# Supplementary material for: Understanding Ion Pairing in High Salt Concentration Electrolytes using Classical Molecular Dynamics Simulations and its Implications for Nonaqueous Li-O$_2$ Batteries
Source: arXiv:1801.09130 source file (2018-01-27)
Supplement: Supplementary file 1 [file supp_info_f.pdf]

# Supplementary Information: Understanding Ion Pairing in High Salt Concentration Electrolytes: Insights from Classical Molecular Dynamics Simulations

**Abhishek Khetan[†,‡], Hamid R. Arjmandi[†], Vikram Pande[‡], Heinz Pitsch[†] and Venkatasubramanian Viswanathan[*,‡]**

**[†] Institute for Combustion Technology, RWTH, Aachen, Germany, 52056**
**[‡] Department of Mechanical Engineering, Carnegie Mellon University, Pittsburgh, Pennsylvania, 15213**
**[*] E-mail: venkvis@cmu.edu**

A. **Figure S1: Plots for normalized radial distribution function, cumulative Values and radially contained ionic charge for all solvent-anion combination considered in the present study.**

<table>
<tr><th>Solvent - Salt</th><th>Normalized radial distribution function</th><th>Cumulative values and radially contained ionic charge</th></tr>
<tr><td>ACN-$BF_4^-$</td><td>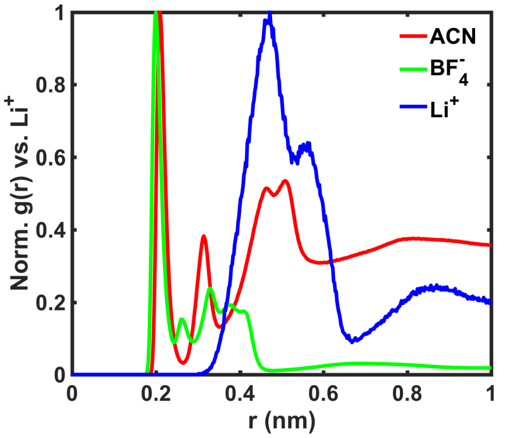
</td><td>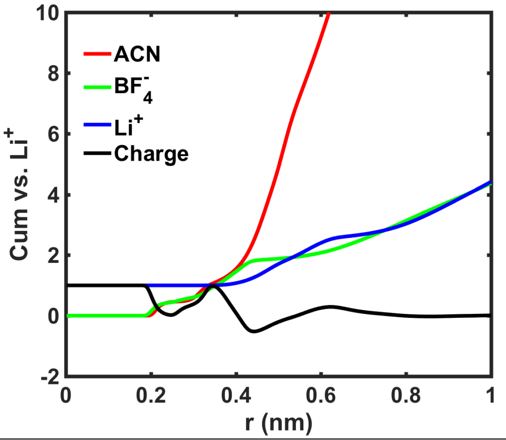
</td></tr>
<tr><td>ACN-$NO_3^-$</td><td>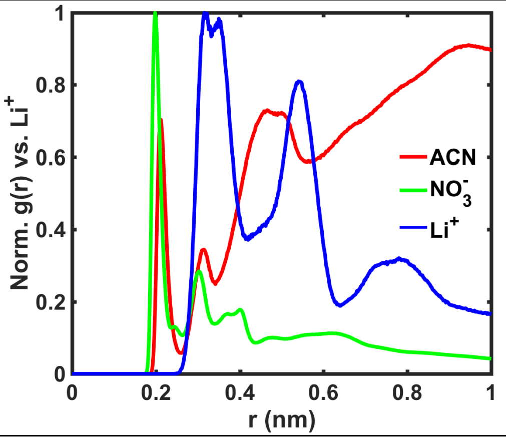
</td><td>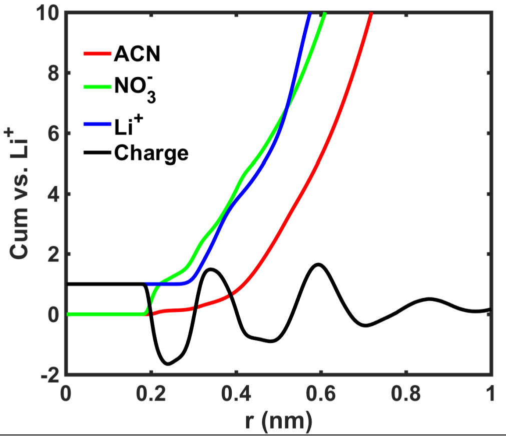
</td></tr>
</table>

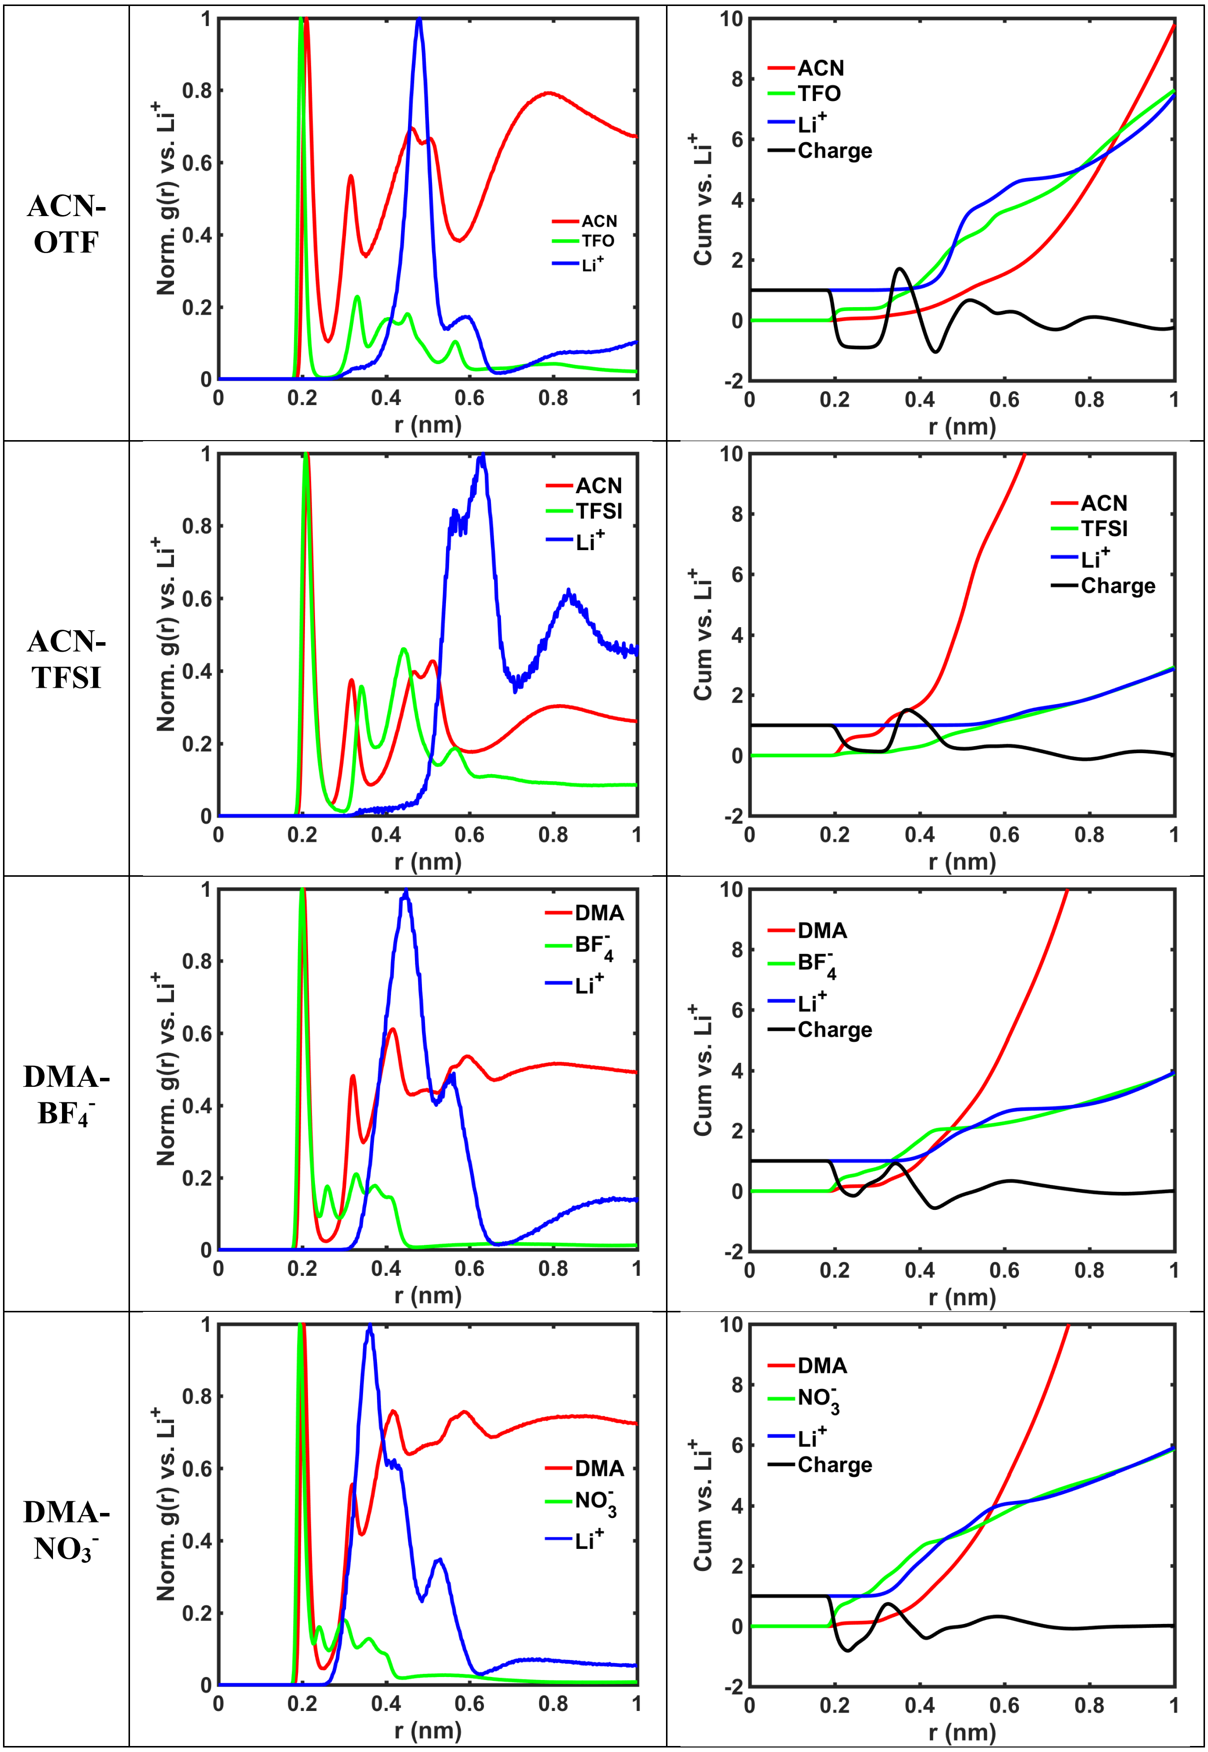

ACN-OTF
ACN-TFSI
DMA-BF4-
DMA-NO3-
Norm. g(r) vs. Li+
Cum vs. Li+
r (nm)
ACN
TFO
TFSI
DMA
BF-4
NO-3
Li+
Charge

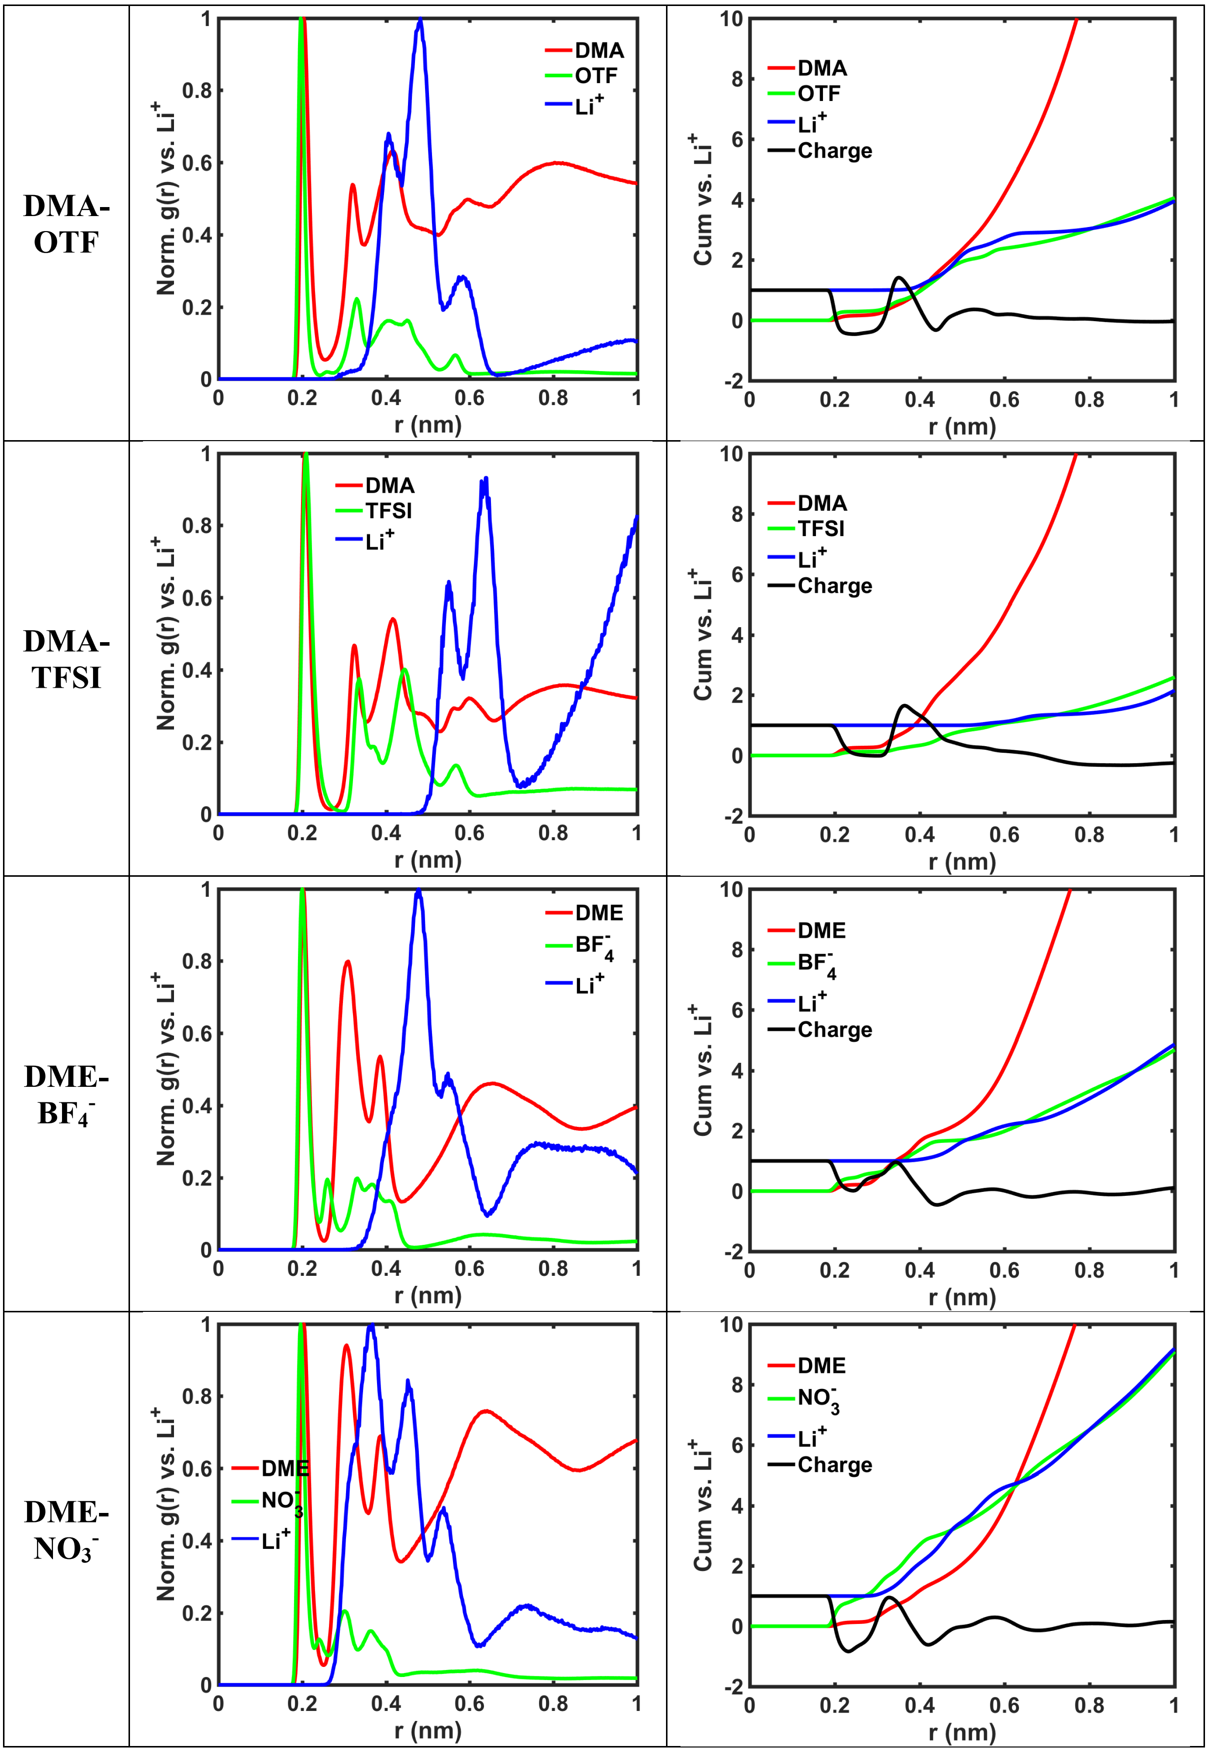
DMA-OTF
DMA-TFSI
DME-BF4-
DME-NO3-
Norm. g(r) vs. Li+
Cum vs. Li+
r (nm)
DMA
OTF
TFSI
DME
BF4-
NO3-
Li+
Charge

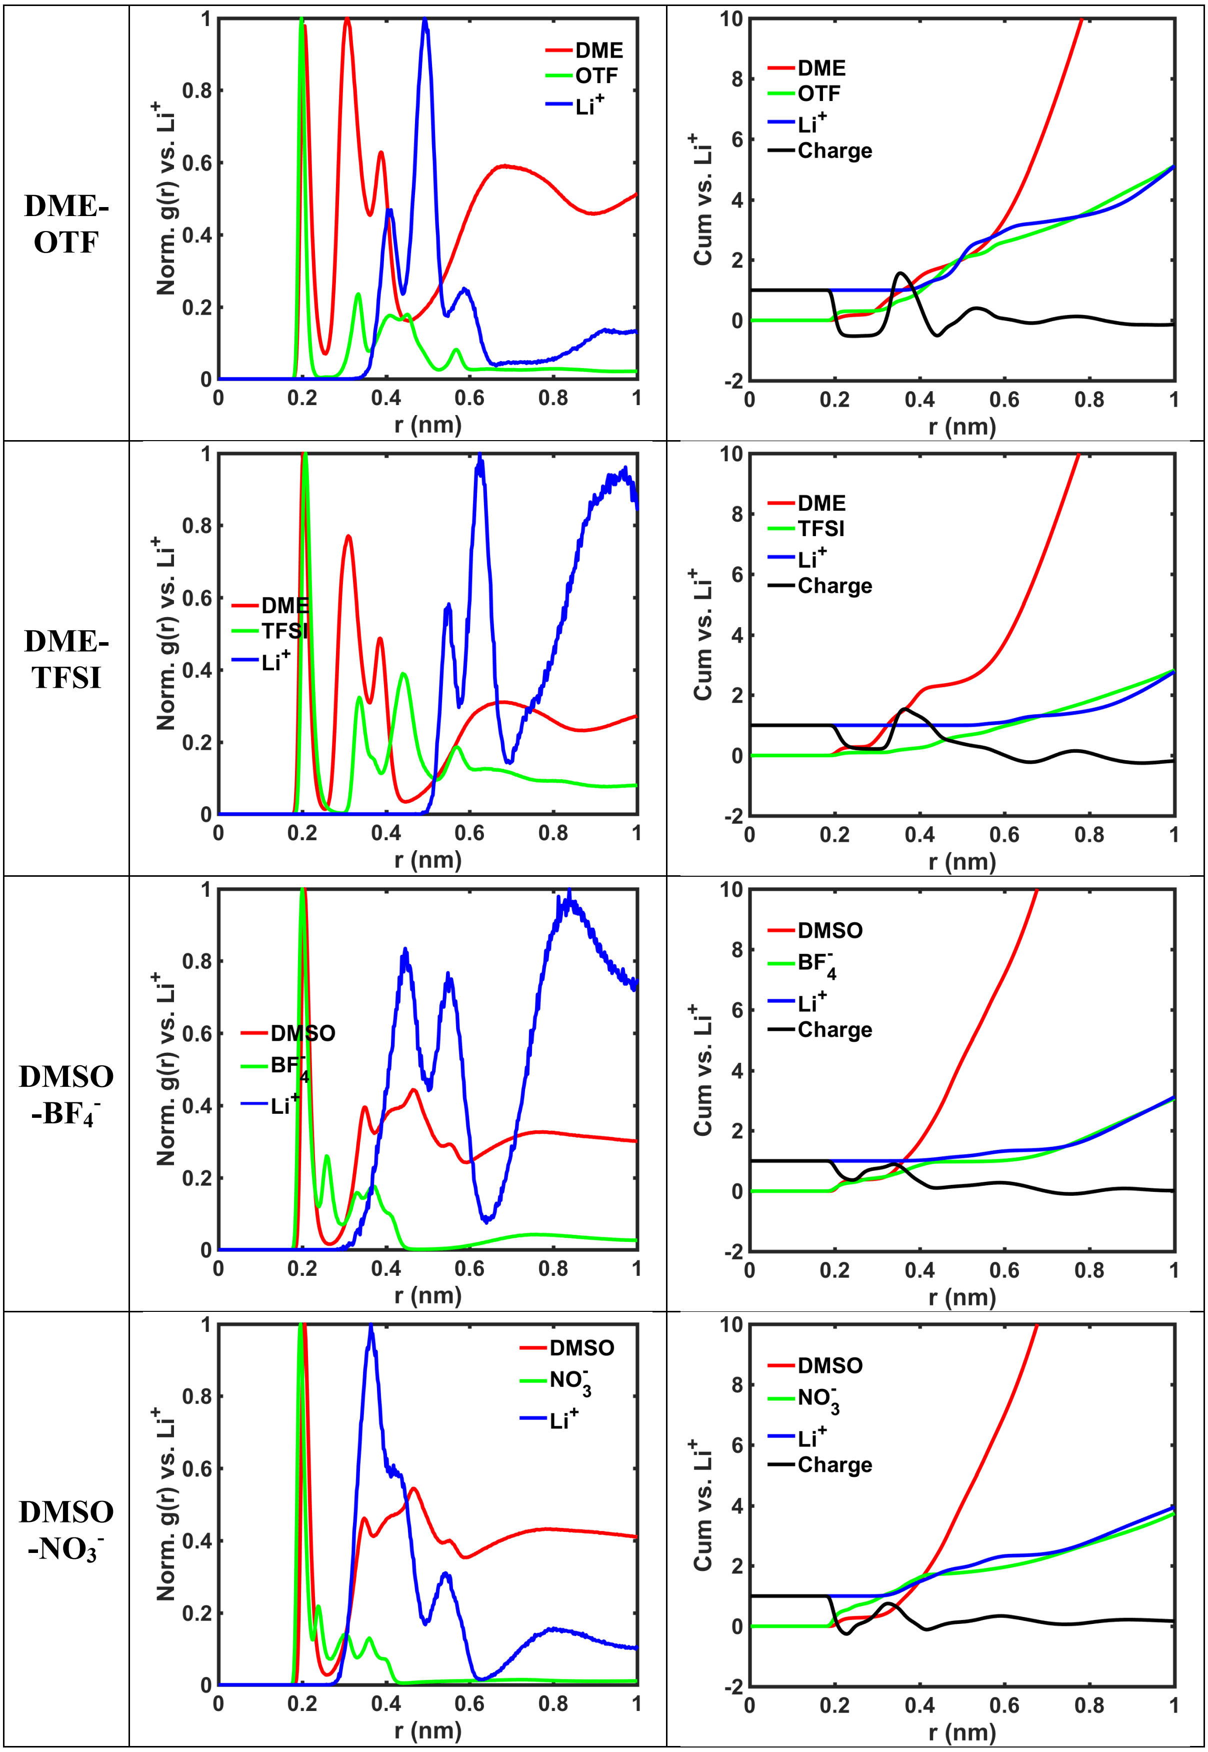
DME-OTF
DME-TFSI
DMSO-$BF_4^-$
DMSO-$NO_3^-$
Norm. g(r) vs. $Li^+$
Cum vs. $Li^+$
r (nm)
DME
OTF
TFSI
DMSO
$BF_4^-$
$NO_3^-$
$Li^+$
Charge

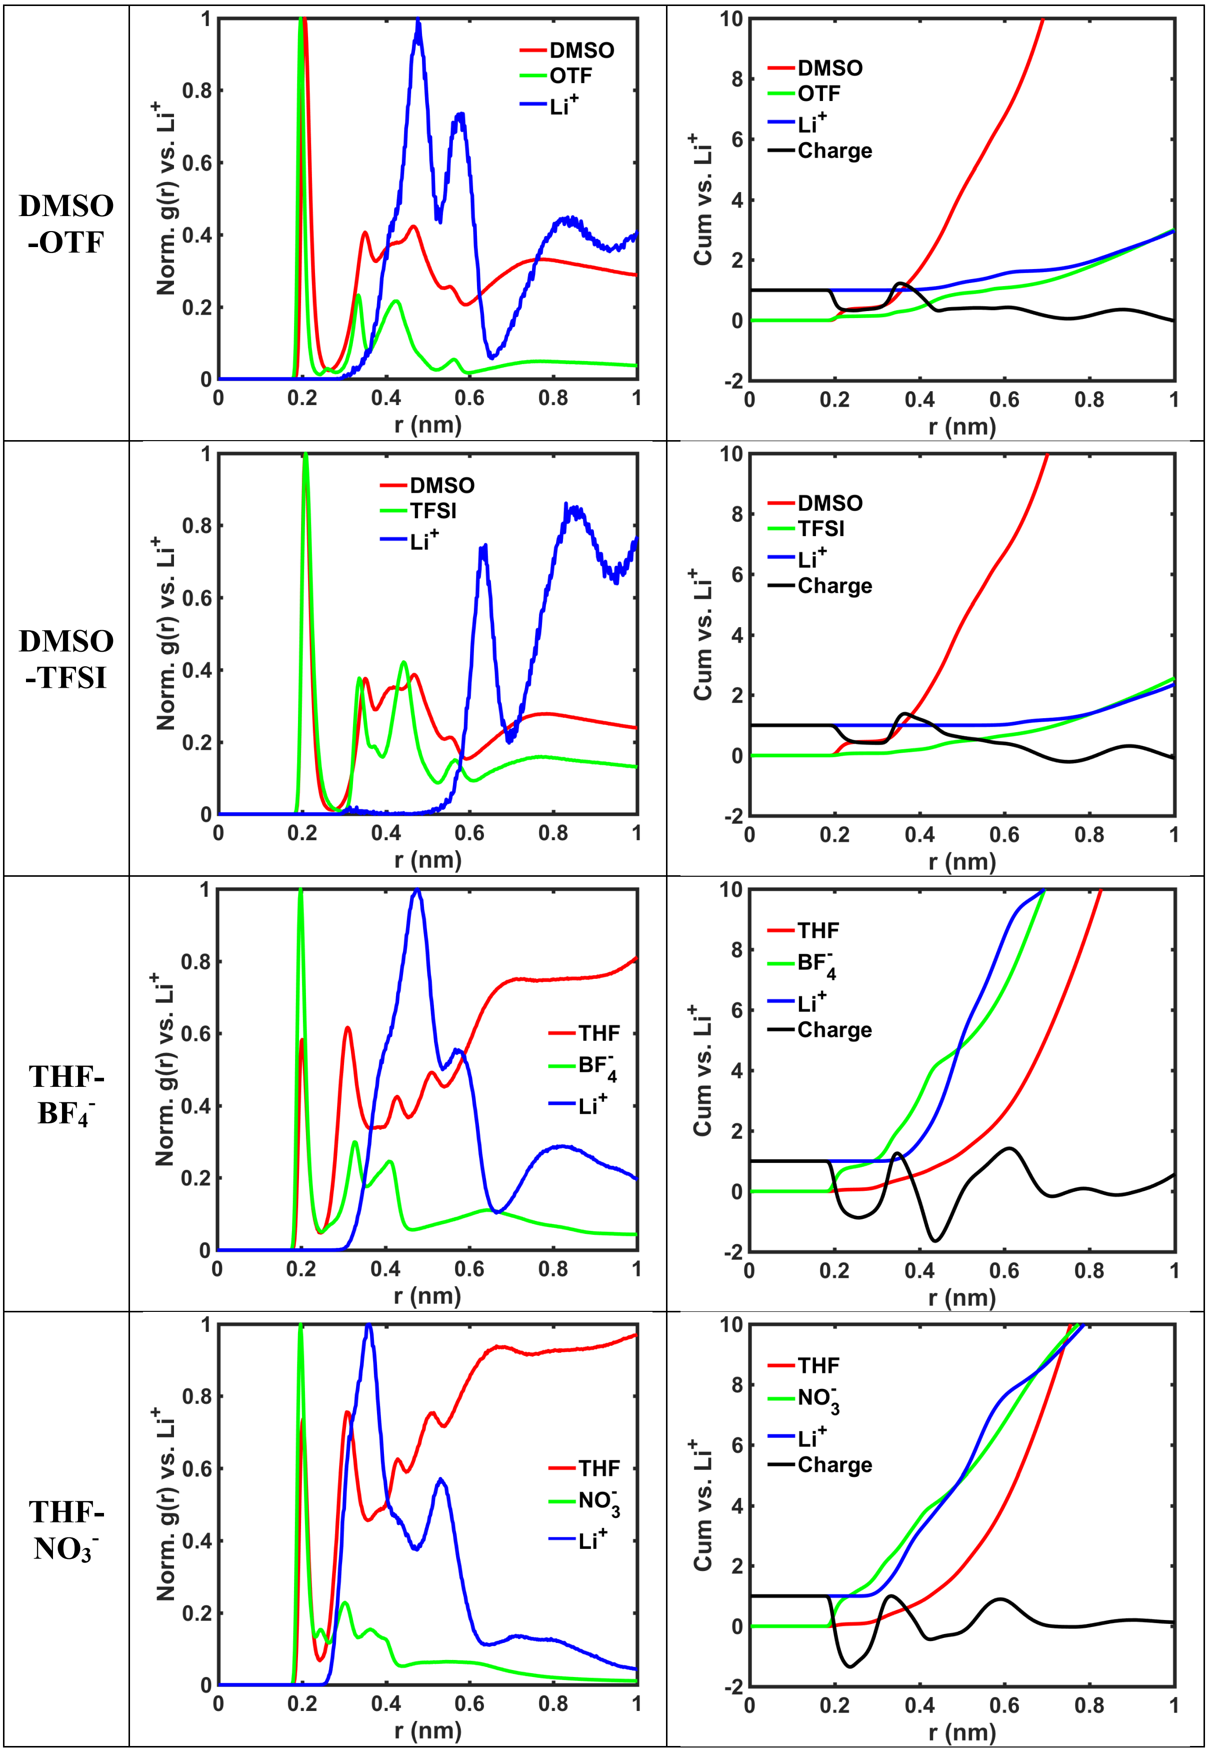

DMSO
-OTF
DMSO
-TFSI
THF-
BF4-
THF-
NO3-
Norm. g(r) vs. Li+
Cum vs. Li+
r (nm)
DMSO
OTF
TFSI
Li+
Charge
THF
BF-4
NO-3

**THF-OTF**

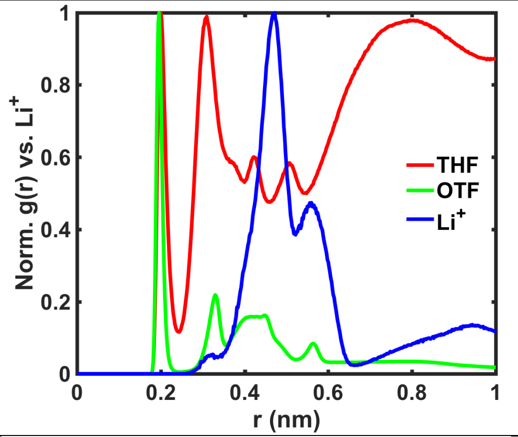


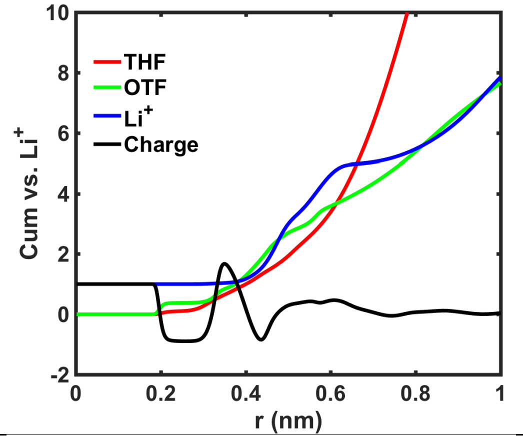


**THF-TFSI**

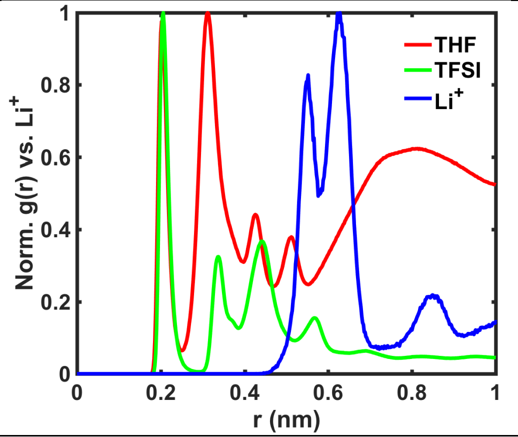


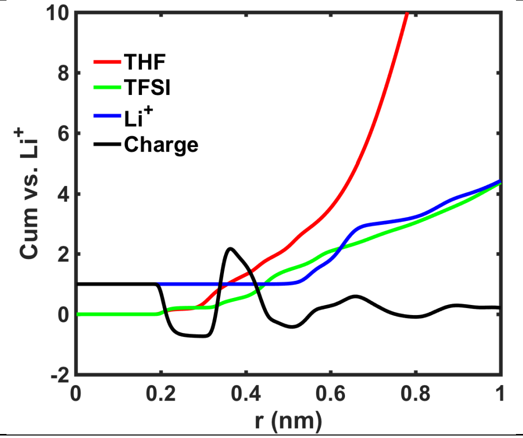


**ACN -(0.1 $NO_3^-$ +0.9 TFSI)**

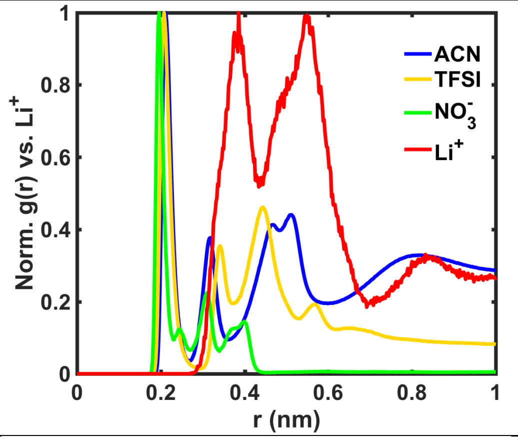


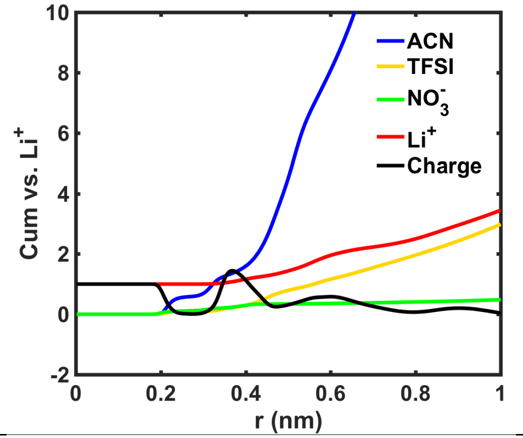


**ACN -(0.2 $NO_3^-$ +0.8 TFSI)**

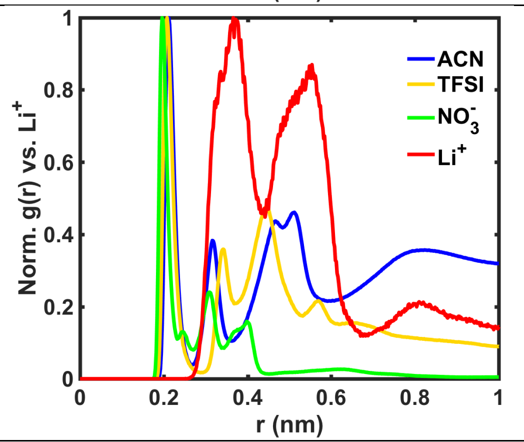


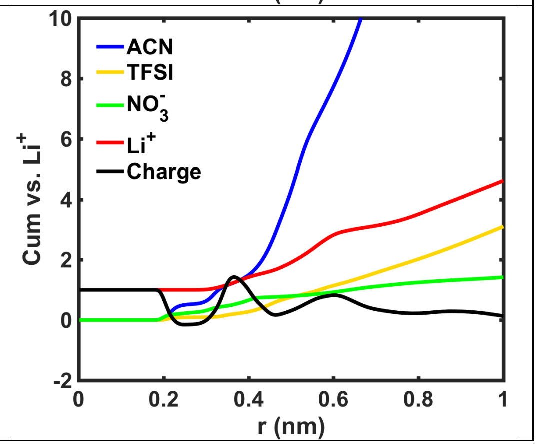

| | | |
|---|---|---|
| ACN -(0.3 $NO_3^-$ +0.7 TFSI) | 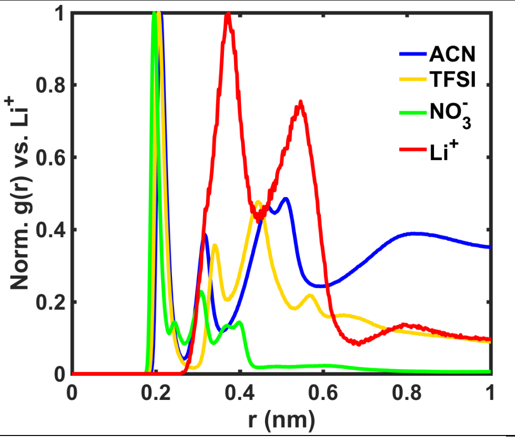 | 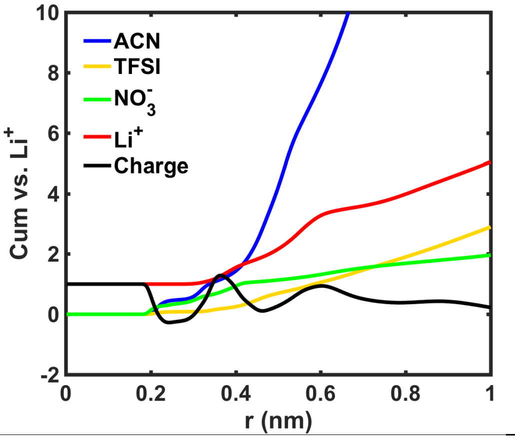 |
| ACN -(0.4 $NO_3^-$ +0.6 TFSI) | 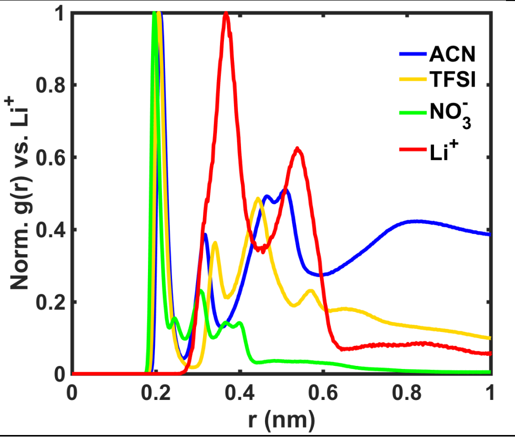 | 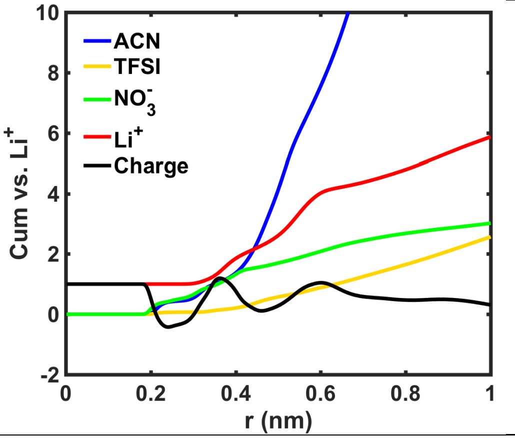 |
| ACN -(0.5 $NO_3^-$ +0.5 TFSI) | 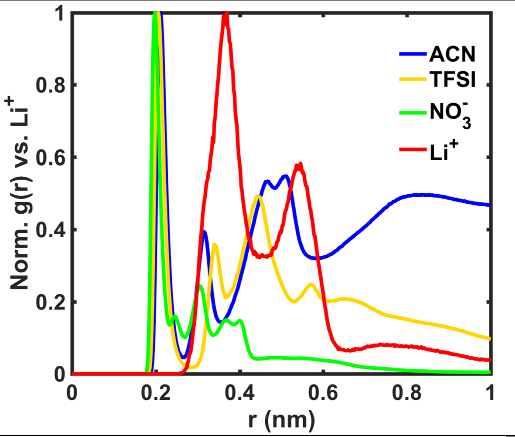 | 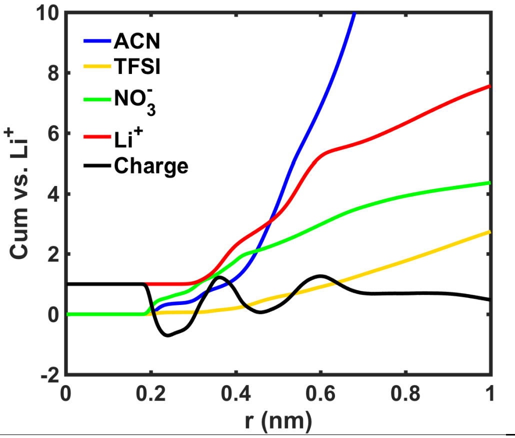 |
| ACN -(0.75 $NO_3^-$ +0.25 TFSI) | 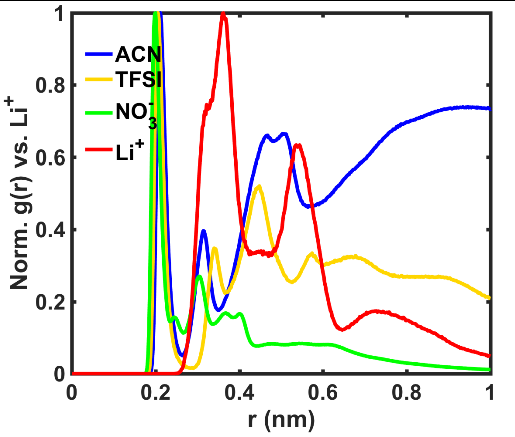 | 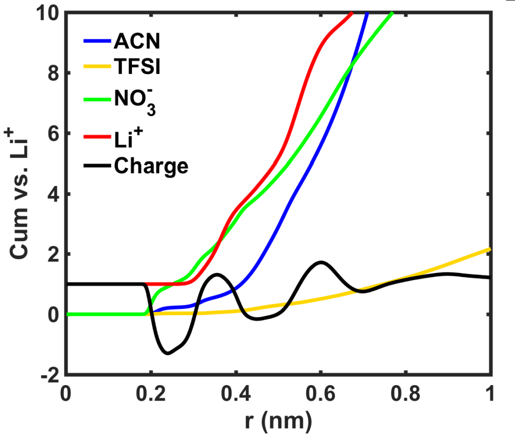 |

DME -(0.1 $NO_3^-$ +0.9 TFSI)

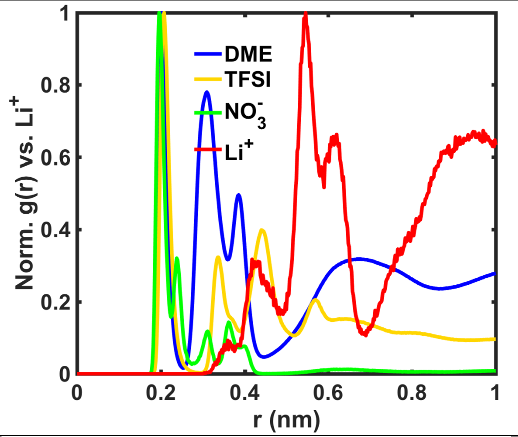


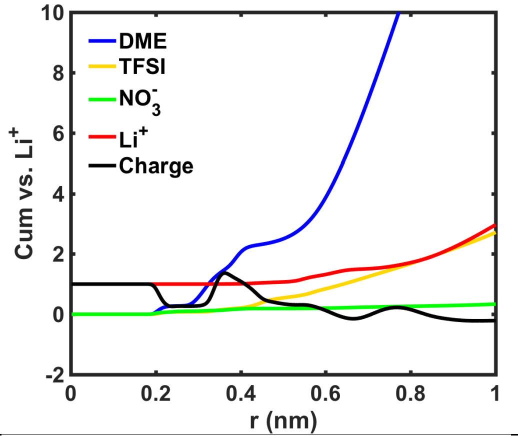


DME -(0.2 $NO_3^-$ +0.8 TFSI)

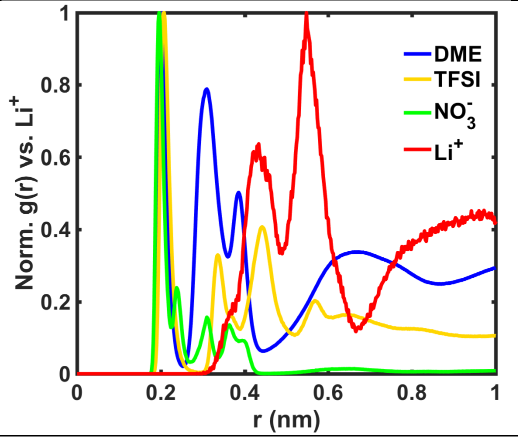


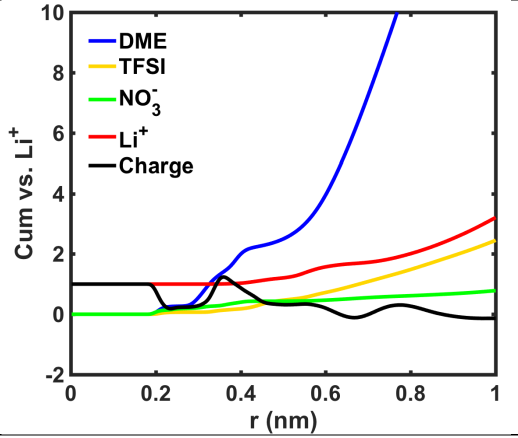


DME -(0.3 $NO_3^-$ +0.7 TFSI)

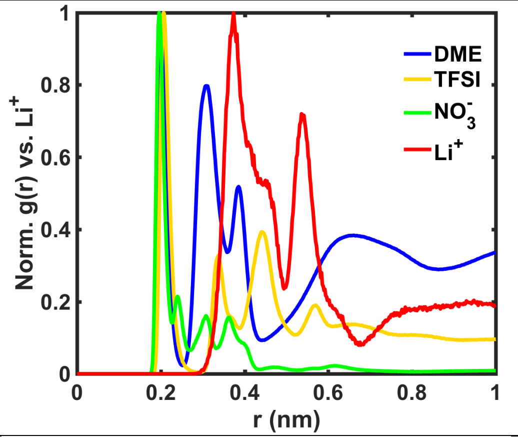


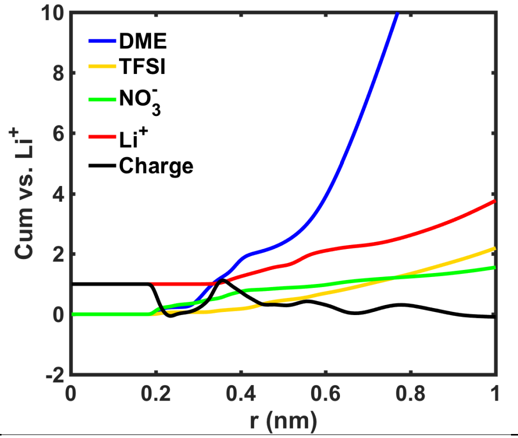


DME -(0.4 $NO_3^-$ +0.6 TFSI)

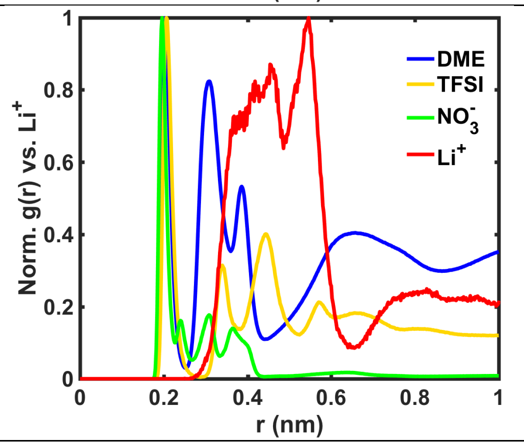


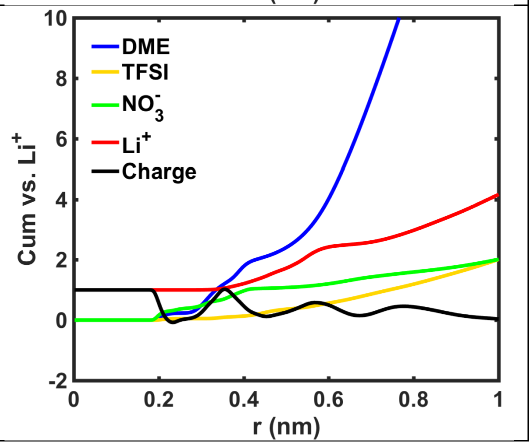

| | | |
|---|---|---|
| DME -(0.5 $NO_3^-$ +0.5 TFSI) | 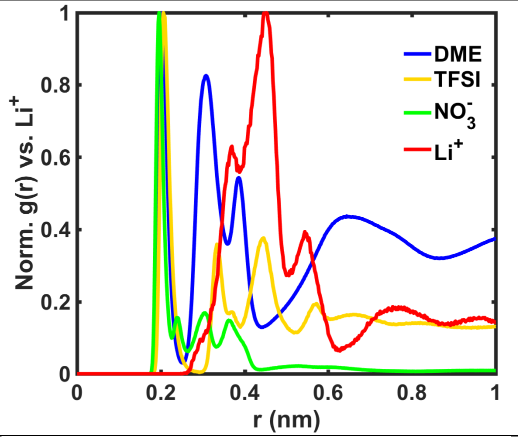 | 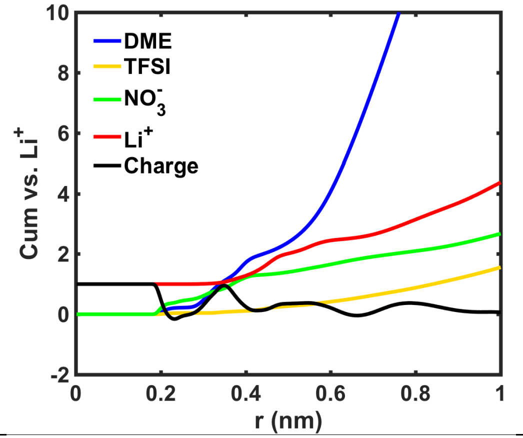 |
| DME -(0.75 $NO_3^-$ +0.25 TFSI) | 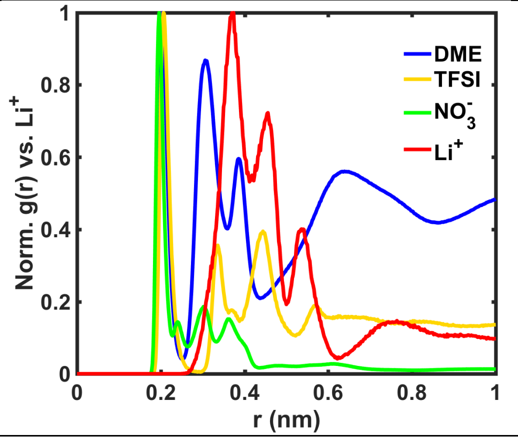 | 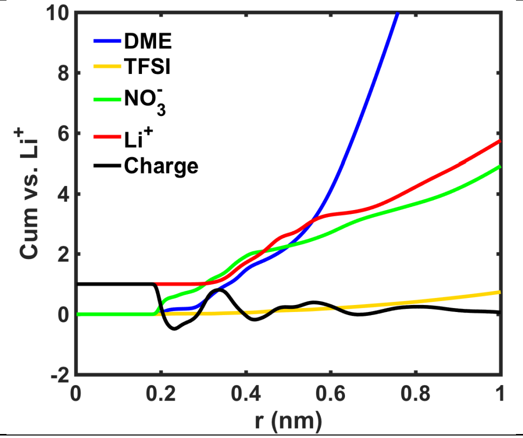 |
| DMSO -(0.1 $NO_3^-$ +0.9 TFSI) | 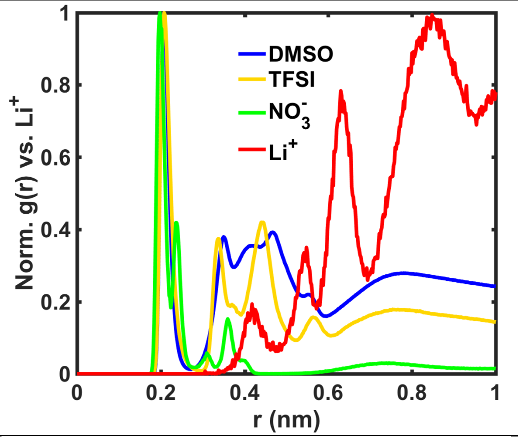 | 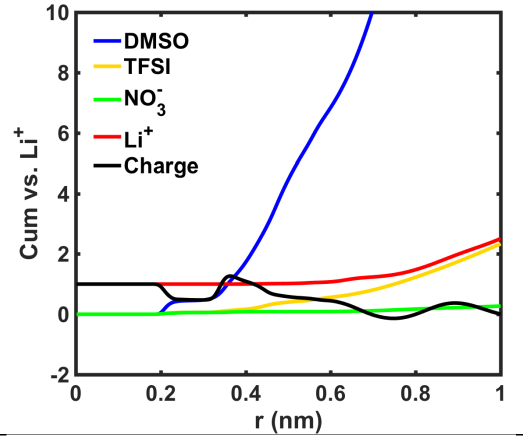 |
| DMSO -(0.2 $NO_3^-$ +0.8 TFSI) | 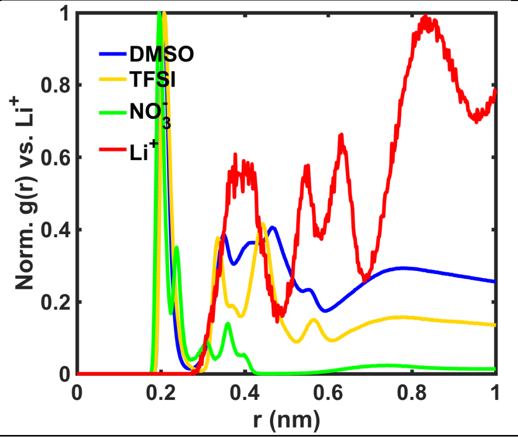 | 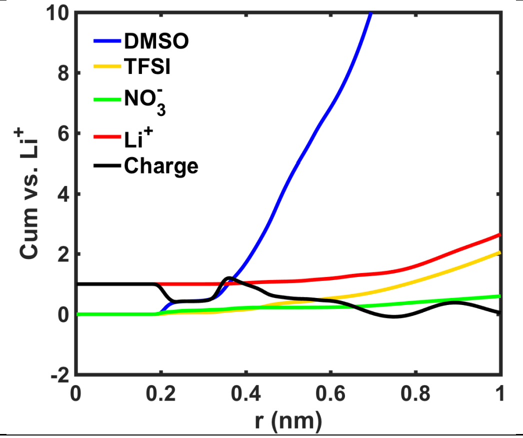 |

**DMSO -(0.3 $NO_3^-$ +0.7 TFSI)**

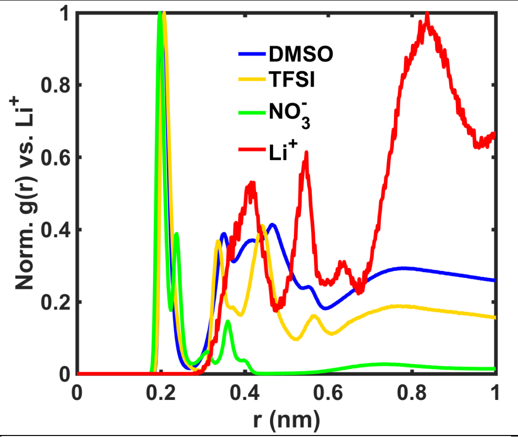


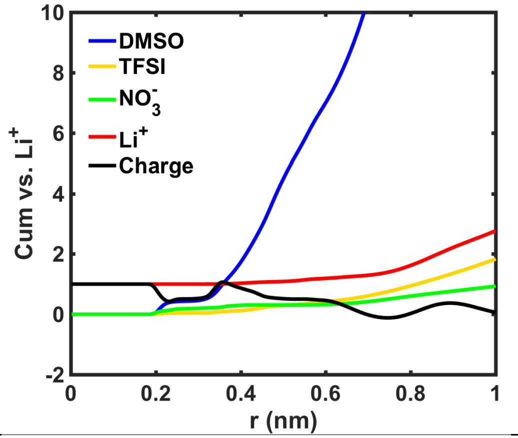


**DMSO -(0.4 $NO_3^-$ +0.6 TFSI)**

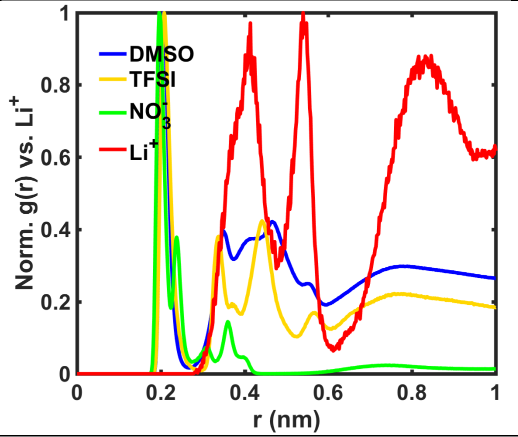


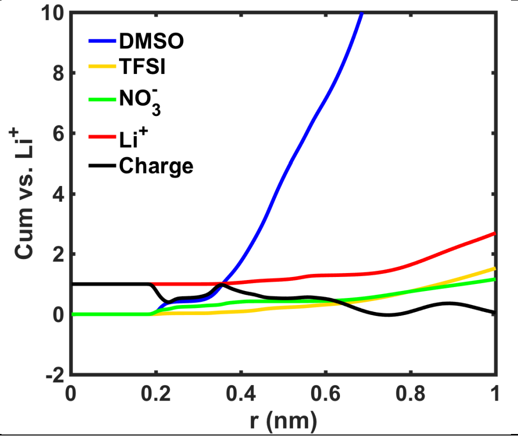


**DMSO -(0.5 $NO_3^-$ +0.5 TFSI)**

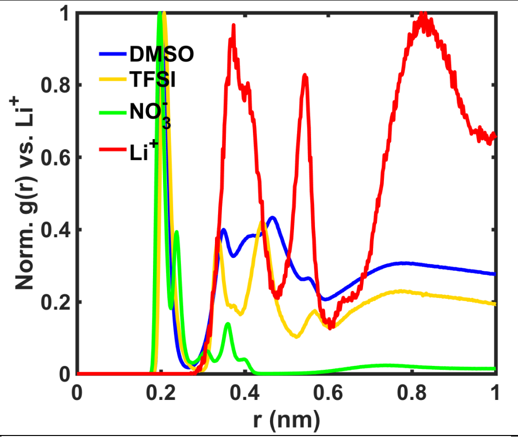


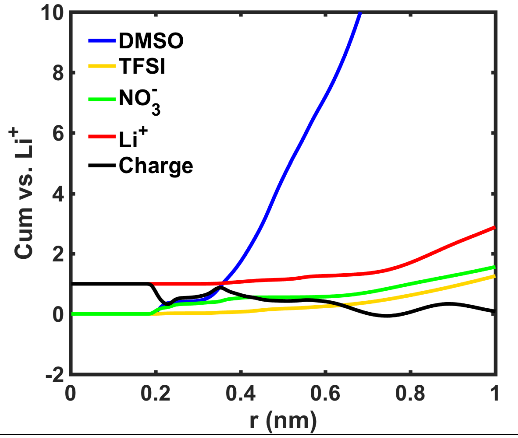


**DMSO -(0.75 $NO_3^-$ +0.25 TFSI)**

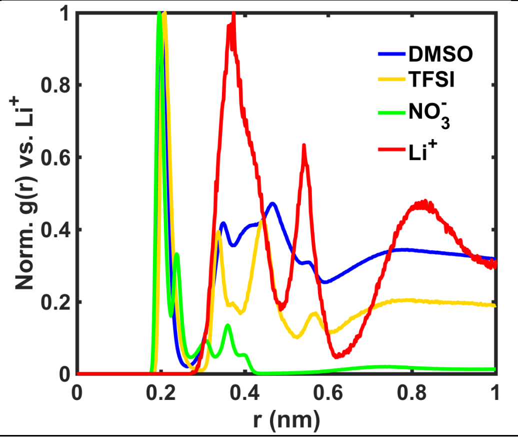


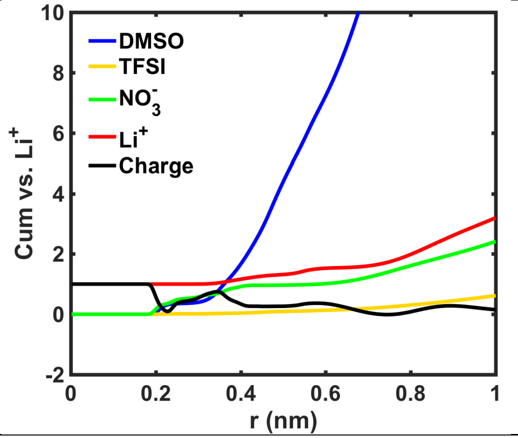

**B. Table S1: Cumulative numbers of $Li^+$ ions, solvent molecules and anions in the ionic cluster (CL) defined by the cutoff limit $r_{cl}$ for 1M mixtures of $NO_3^-$+TFSI in solvents ACN, DME and DMSO**

| Solvent | Fraction of $NO_3^-$ | $r_{cl}$ Cutoff of CL (nm) | No. of Solvents in CL | No. of $Li^+$ in CL | No. of $NO_3^-$ in CL | No. of TFSI in CL |
|---|---|---|---|---|---|---|
| ACN | 0.000 | 0.696 | 12.110 | 1.585 | 0.000 | 1.480 |
| | 0.100 | 0.710 | 12.030 | 2.229 | 0.379 | 1.545 |
| | 0.200 | 0.694 | 10.050 | 3.117 | 1.103 | 1.537 |
| | 0.300 | 0.694 | 11.370 | 3.576 | 1.526 | 1.439 |
| | 0.400 | 0.710 | 12.300 | 4.407 | 2.470 | 1.288 |
| | 0.500 | 0.732 | 12.890 | 5.888 | 3.689 | 1.463 |
| | 0.750 | 0.798 | 15.630 | 12.660 | 10.440 | 1.195 |
| | 1.000 | 0.910 | 24.310 | 22.950 | 22.700 | 0.000 |
| DME | 0.000 | 0.716 | 7.580 | 1.339 | 0.000 | 1.445 |
| | 0.100 | 0.716 | 7.730 | 1.524 | 0.241 | 1.315 |
| | 0.200 | 0.610 | 4.222 | 1.596 | 0.475 | 0.753 |
| | 0.300 | 0.612 | 4.223 | 2.139 | 0.999 | 0.730 |
| | 0.400 | 0.620 | 4.524 | 2.460 | 1.241 | 0.608 |
| | 0.500 | 0.608 | 4.296 | 2.461 | 1.675 | 0.430 |
| | 0.750 | 0.612 | 4.466 | 3.319 | 2.788 | 0.205 |
| | 1.000 | 0.628 | 4.807 | 4.739 | 4.682 | 0.000 |
| DMSO | 0.000 | 0.824 | 17.310 | 1.480 | 0.000 | 1.459 |
| | 0.100 | 0.822 | 17.370 | 1.577 | 0.185 | 1.337 |
| | 0.200 | 0.674 | 9.106 | 1.307 | 0.266 | 0.663 |
| | 0.300 | 0.666 | 8.997 | 1.257 | 0.374 | 0.529 |
| | 0.400 | 0.654 | 8.738 | 1.307 | 0.480 | 0.388 |
| | 0.500 | 0.650 | 8.719 | 1.297 | 0.623 | 0.308 |
| | 0.750 | 0.544 | 5.630 | 1.413 | 0.977 | 0.107 |
| | 1.000 | 0.504 | 4.163 | 1.959 | 1.783 | 0.000 |

## C. Table S2: Coordination numbers (CN), cumulative numbers of $Li^+$ ions, solvent molecules and anions in the ionic cluster (CL) defined by the cutoff limit $r_{cl}$ for all salt anion-solvent combinations considered in this work.

| Anion | Solvent | CN of Anion vs. $Li^+$ | CN of Solvent vs. $Li^+$ | $r_{cl}$ Cutoff of CL (nm) | No. of Solvents in CL | No. of $Li^+$ in CL | No. of Anions in CL |
|---|---|---|---|---|---|---|---|
| $NO_3^-$ | ACN | 1.125 | 0.113 | 0.910 | 24.310 | 22.950 | 22.700 |
| $NO_3^-$ | DMSO | 0.532 | 0.245 | 0.504 | 4.163 | 1.959 | 1.783 |
| $NO_3^-$ | THF | 0.992 | 0.072 | 0.830 | 13.930 | 10.700 | 10.730 |
| $NO_3^-$ | DMA | 0.758 | 0.102 | 0.670 | 6.917 | 4.186 | 4.236 |
| $NO_3^-$ | DME | 0.769 | 0.119 | 0.628 | 4.807 | 4.739 | 4.682 |
| TFSI | ACN | 0.110 | 0.738 | 0.696 | 12.110 | 1.585 | 1.480 |
| TFSI | DMSO | 0.074 | 0.466 | 0.824 | 17.310 | 1.480 | 1.459 |
| TFSI | THF | 0.218 | 0.263 | 0.848 | 13.950 | 3.526 | 3.315 |
| TFSI | DMA | 0.127 | 0.277 | 0.732 | 8.470 | 1.358 | 1.376 |
| TFSI | DME | 0.099 | 0.444 | 0.716 | 7.580 | 1.339 | 1.445 |
| OTF | ACN | 0.377 | 0.241 | 0.766 | 3.806 | 4.954 | 4.883 |
| OTF | DMSO | 0.134 | 0.379 | 0.676 | 9.331 | 1.644 | 1.223 |
| OTF | THF | 0.376 | 0.101 | 0.808 | 11.470 | 5.523 | 5.481 |
| OTF | DMA | 0.290 | 0.154 | 0.730 | 8.214 | 2.938 | 2.726 |
| OTF | DME | 0.484 | 0.171 | 0.716 | 7.159 | 3.307 | 3.118 |
| $BF_4^-$ | ACN | 0.433 | 0.443 | 0.742 | 17.140 | 2.796 | 2.774 |
| $BF_4^-$ | DMSO | 0.285 | 0.362 | 0.516 | 4.799 | 1.170 | 0.979 |
| $BF_4^-$ | THF | 0.797 | 0.069 | 0.766 | 7.378 | 11.390 | 12.480 |
| $BF_4^-$ | DMA | 0.511 | 0.160 | 0.730 | 9.215 | 2.761 | 2.680 |
| $BF_4^-$ | DME | 0.435 | 0.206 | 0.618 | 4.666 | 2.217 | 2.090 |

**D. GROMACS Forcefield parameters for various all solvents:**

1. DMA ($C_4H_9NO$)

[ atoms ]

| | | | | | | | |
|---|---|---|---|---|---|---|---|
| 1 | opls_135 | 1 | DMA | C | 1 | -0.18 | 12.011 |
| 2 | opls_282 | 1 | DMA | H | 2 | 0.06 | 1.008 |
| 3 | opls_282 | 1 | DMA | H | 3 | 0.06 | 1.008 |
| 4 | opls_282 | 1 | DMA | H | 4 | 0.06 | 1.008 |
| 5 | opls_235 | 1 | DMA | C | 5 | 0.5 | 12.011 |
| 6 | opls_236 | 1 | DMA | O | 6 | -0.5 | 15.9994 |
| 7 | opls_239 | 1 | DMA | N | 7 | -0.14 | 14.0067 |
| 8 | opls_243 | 1 | DMA | C | 8 | -0.11 | 12.011 |
| 9 | opls_282 | 1 | DMA | H | 9 | 0.06 | 1.008 |
| 10 | opls_282 | 1 | DMA | H | 10 | 0.06 | 1.008 |
| 11 | opls_282 | 1 | DMA | H | 11 | 0.06 | 1.008 |
| 12 | opls_243 | 1 | DMA | C | 12 | -0.11 | 12.011 |
| 13 | opls_282 | 1 | DMA | H | 13 | 0.06 | 1.008 |
| 14 | opls_282 | 1 | DMA | H | 14 | 0.06 | 1.008 |
| 15 | opls_282 | 1 | DMA | H | 15 | 0.06 | 1.008 |

[ bonds ]

| | | |
|---|---|---|
| 1 | 2 | 1 |
| 1 | 3 | 1 |
| 1 | 4 | 1 |
| 1 | 5 | 1 |
| 5 | 6 | 1 |
| 5 | 7 | 1 |
| 7 | 8 | 1 |
| 7 | 12 | 1 |
| 8 | 9 | 1 |
| 8 | 10 | 1 |
| 8 | 11 | 1 |
| 12 | 13 | 1 |
| 12 | 14 | 1 |
| 12 | 15 | 1 |

[ pairs ]

| | | |
|---|---|---|
| 1 | 8 | 1 |
| 1 | 12 | 1 |
| 2 | 6 | 1 |
| 2 | 7 | 1 |
| 3 | 6 | 1 |
| 3 | 7 | 1 |
| 4 | 6 | 1 |
| 4 | 7 | 1 |
| 5 | 9 | 1 |
| 5 | 10 | 1 |
| 5 | 11 | 1 |
| 5 | 13 | 1 |
| 5 | 14 | 1 |
| 5 | 15 | 1 |
| 6 | 8 | 1 |
| 6 | 12 | 1 |

8 13 1
8 14 1
8 15 1
9 12 1
10 12 1
11 12 1
[ angles ]
2 1 3 1
2 1 4 1
2 1 5 1
3 1 4 1
3 1 5 1
4 1 5 1
1 5 6 1
1 5 7 1
6 5 7 1
5 7 8 1
5 7 12 1
8 7 12 1
7 8 9 1
7 8 10 1
7 8 11 1
9 8 10 1
9 8 11 1
10 8 11 1
7 12 13 1
7 12 14 1
7 12 15 1
13 12 14 1
13 12 15 1
14 12 15 1
[ dihedrals ]
2 1 5 6 3
2 1 5 7 3
3 1 5 6 3
3 1 5 7 3
4 1 5 6 3
4 1 5 7 3
1 5 7 8 3
1 5 7 12 3
6 5 7 8 3
6 5 7 12 3
5 7 8 9 3
5 7 8 10 3
5 7 8 11 3
12 7 8 9 3
12 7 8 10 3
12 7 8 11 3
5 7 12 13 3
5 7 12 14 3

5 7 12 15 3
8 7 12 13 3
8 7 12 14 3
8 7 12 15 3
; Added DvdS 2010-12-21
5 1 7 6 1 180 4.6 2
5 8 12 7 1 180 4.6 2

2. ACN ($C_2H_3N$)

[ atoms ]

| | | | | | | | |
|---|---|---|---|---|---|---|---|
| 1 | opls_755 | 1 | ACN | C | 1 | -0.08 | 12.01100 |
| 2 | opls_759 | 1 | ACN | H | 1 | 0.06 | 1.00800 |
| 3 | opls_759 | 1 | ACN | H | 1 | 0.06 | 1.00800 |
| 4 | opls_759 | 1 | ACN | H | 1 | 0.06 | 1.00800 |
| 5 | opls_754 | 1 | ACN | C | 2 | 0.46 | 12.01100 |
| 6 | opls_753 | 1 | ACN | N | 3 | -0.56 | 14.00670 |

[ bonds ]
1 2 1
1 3 1
1 4 1
1 5 1
5 6 1
[ angles ]
2 1 3 1
2 1 4 1
2 1 5 1
3 1 4 1
3 1 5 1
4 1 5 1
1 5 6 1
[ dihedrals ]
2 1 5 6 3
3 1 5 6 3
4 1 5 6 3
[ pairs ]
2 6 1
3 6 1
4 6 1

3. THF ($C_4H_8O$)

[ atoms ]

| | | | | | | | |
|---|---|---|---|---|---|---|---|
| 1 | opls_182 | 1 | THF | C | 1 | 0.14 | 12.011 |
| 2 | opls_185 | 1 | THF | H | 2 | 0.03 | 1.008 |
| 3 | opls_185 | 1 | THF | H | 3 | 0.03 | 1.008 |
| 4 | opls_136 | 1 | THF | C | 4 | -0.12 | 12.011 |
| 5 | opls_140 | 1 | THF | H | 5 | 0.06 | 1.008 |
| 6 | opls_140 | 1 | THF | H | 6 | 0.06 | 1.008 |
| 7 | opls_136 | 1 | THF | C | 7 | -0.12 | 12.011 |

```
8   opls_140        1       THF        H        8      0.06     1.008
9   opls_140        1       THF        H        9      0.06     1.008
10   opls_182        1       THF        C        10      0.14    12.011
11   opls_185        1       THF        H        11      0.03     1.008
12   opls_185        1       THF        H        12      0.03     1.008
13   opls_180        1       THF        O        13      -0.4   15.9994
[ bonds ]
    1     2     1
    1     3     1
    1     4     1
    1    13     1
    4     5     1
    4     6     1
    4     7     1
    7     8     1
    7     9     1
    7    10     1
   10    11     1
   10    12     1
   10    13     1
 [ pairs ]
    1     8     1
    1     9     1
    1    11     1
    1    12     1
    2     5     1
    2     6     1
    2     7     1
    2    10     1
    3     5     1
    3     6     1
    3     7     1
    3    10     1
    4    11     1
    4    12     1
    5     8     1
    5     9     1
    5    10     1
    5    13     1
    6     8     1
    6     9     1
    6    10     1
    6    13     1
    8    11     1
    8    12     1
    8    13     1
    9    11     1
    9    12     1
    9    13     1
 [ angles ]
```

```
   2    1    3    1
   2    1    4    1
   2    1   13    1
   3    1    4    1
   3    1   13    1
   4    1   13    1
   1    4    5    1
   1    4    6    1
   1    4    7    1
   5    4    6    1
   5    4    7    1
   6    4    7    1
   4    7    8    1
   4    7    9    1
   4    7   10    1
   8    7    9    1
   8    7   10    1
   9    7   10    1
   7   10   11    1
   7   10   12    1
   7   10   13    1
  11   10   12    1
  11   10   13    1
  12   10   13    1
   1   13   10    1
[ dihedrals ]
   2    1    4    5    3
   2    1    4    6    3
   2    1    4    7    3
   3    1    4    5    3
   3    1    4    6    3
   3    1    4    7    3
  13    1    4    5    3
  13    1    4    6    3
  13    1    4    7    3
   2    1   13   10    3
   3    1   13   10    3
   4    1   13   10    3
   1    4    7    8    3
   1    4    7    9    3
   1    4    7   10    3
   5    4    7    8    3
   5    4    7    9    3
   5    4    7   10    3
   6    4    7    8    3
   6    4    7    9    3
   6    4    7   10    3
   4    7   10   11    3
   4    7   10   12    3
   4    7   10   13    3
```

| | | | | |
|---|---|---|---|---|
| 8 | 7 | 10 | 11 | 3 |
| 8 | 7 | 10 | 12 | 3 |
| 8 | 7 | 10 | 13 | 3 |
| 9 | 7 | 10 | 11 | 3 |
| 9 | 7 | 10 | 12 | 3 |
| 9 | 7 | 10 | 13 | 3 |
| 7 | 10 | 13 | 1 | 3 |
| 11 | 10 | 13 | 1 | 3 |
| 12 | 10 | 13 | 1 | 3 |

4. DMSO ($C_2H_6OS$)

[ atoms ]

| | | | | | | | |
|---|---|---|---|---|---|---|---|
| 1 | opls_498 | 1 | DMS | C | 1 | -0.035 | 12.011 |
| 2 | opls_140 | 1 | DMS | H | 2 | 0.06 | 1.008 |
| 3 | opls_140 | 1 | DMS | H | 3 | 0.06 | 1.008 |
| 4 | opls_140 | 1 | DMS | H | 4 | 0.06 | 1.008 |
| 5 | opls_496 | 1 | DMS | S | 5 | 0.13 | 32.06 |
| 6 | opls_498 | 1 | DMS | C | 6 | -0.035 | 12.011 |
| 7 | opls_140 | 1 | DMS | H | 7 | 0.06 | 1.008 |
| 8 | opls_140 | 1 | DMS | H | 8 | 0.06 | 1.008 |
| 9 | opls_140 | 1 | DMS | H | 9 | 0.06 | 1.008 |
| 10 | opls_497 | 1 | DMS | O | 10 | -0.42 | 15.9994 |

[ bonds ]

| | | |
|---|---|---|
| 1 | 2 | 1 |
| 1 | 3 | 1 |
| 1 | 4 | 1 |
| 1 | 5 | 1 |
| 5 | 6 | 1 |
| 5 | 10 | 1 |
| 6 | 7 | 1 |
| 6 | 8 | 1 |
| 6 | 9 | 1 |

[ pairs ]

| | | |
|---|---|---|
| 1 | 7 | 1 |
| 1 | 8 | 1 |
| 1 | 9 | 1 |
| 2 | 6 | 1 |
| 2 | 10 | 1 |
| 3 | 6 | 1 |
| 3 | 10 | 1 |
| 4 | 6 | 1 |
| 4 | 10 | 1 |
| 7 | 10 | 1 |
| 8 | 10 | 1 |
| 9 | 10 | 1 |

[ angles ]

| | | | |
|---|---|---|---|
| 2 | 1 | 3 | 1 |
| 2 | 1 | 4 | 1 |
| 2 | 1 | 5 | 1 |

| | | | |
|---|---|---|---|
| 3 | 1 | 4 | 1 |
| 3 | 1 | 5 | 1 |
| 4 | 1 | 5 | 1 |
| 1 | 5 | 6 | 1 |
| 1 | 5 | 10 | 1 |
| 6 | 5 | 10 | 1 |
| 5 | 6 | 7 | 1 |
| 5 | 6 | 8 | 1 |
| 5 | 6 | 9 | 1 |
| 7 | 6 | 8 | 1 |
| 7 | 6 | 9 | 1 |
| 8 | 6 | 9 | 1 |

[ dihedrals ]

| | | | | |
|---|---|---|---|---|
| 2 | 1 | 5 | 6 | 3 |
| 2 | 1 | 5 | 10 | 3 |
| 3 | 1 | 5 | 6 | 3 |
| 3 | 1 | 5 | 10 | 3 |
| 4 | 1 | 5 | 6 | 3 |
| 4 | 1 | 5 | 10 | 3 |
| 1 | 5 | 6 | 7 | 3 |
| 1 | 5 | 6 | 8 | 3 |
| 1 | 5 | 6 | 9 | 3 |
| 10 | 5 | 6 | 7 | 3 |
| 10 | 5 | 6 | 8 | 3 |
| 10 | 5 | 6 | 9 | 3 |

5. DME ($C_4H_{10}O_2$)

[ atoms ]

| | | | | | | | |
|---|---|---|---|---|---|---|---|
| 1 | opls_181 | 1 | DME | C | 1 | 0.110 | 12.01100 |
| 2 | opls_180 | 1 | DME | O | 1 | -0.400 | 15.99940 |
| 3 | opls_185 | 1 | DME | H | 1 | 0.030 | 1.00800 |
| 4 | opls_185 | 1 | DME | H | 1 | 0.030 | 1.00800 |
| 5 | opls_185 | 1 | DME | H | 1 | 0.030 | 1.00800 |
| 6 | opls_180 | 1 | DME | O | 7 | -0.400 | 15.99940 |
| 7 | opls_181 | 1 | DME | C | 7 | 0.110 | 12.01100 |
| 8 | opls_185 | 1 | DME | H | 7 | 0.030 | 1.00800 |
| 9 | opls_185 | 1 | DME | H | 7 | 0.030 | 1.00800 |
| 10 | opls_185 | 1 | DME | H | 7 | 0.030 | 1.00800 |
| 11 | opls_182 | 1 | DME | C | 13 | 0.140 | 12.01100 |
| 12 | opls_185 | 1 | DME | H | 13 | 0.030 | 1.00800 |
| 13 | opls_185 | 1 | DME | H | 13 | 0.030 | 1.00800 |
| 14 | opls_182 | 1 | DME | C | 15 | 0.140 | 12.01100 |
| 15 | opls_185 | 1 | DME | H | 15 | 0.030 | 1.00800 |
| 16 | opls_185 | 1 | DME | H | 15 | 0.030 | 1.00800 |

[ bonds ]

| | | |
|---|---|---|
| 1 | 2 | 1 |
| 1 | 3 | 1 |
| 1 | 4 | 1 |
| 1 | 5 | 1 |

2 11 1
11 14 1
11 12 1
11 13 1
14 6 1
14 15 1
14 16 1
6 7 1
7 8 1
7 9 1
7 10 1
[ angles ]
2 1 3 1
2 1 4 1
2 1 5 1
3 1 4 1
3 1 5 1
4 1 5 1
1 2 11 1
2 11 14 1
2 11 12 1
2 11 13 1
14 11 12 1
14 11 13 1
12 11 13 1
11 14 6 1
11 14 15 1
11 14 16 1
6 14 15 1
6 14 16 1
15 14 16 1
14 6 7 1
6 7 8 1
6 7 9 1
6 7 10 1
8 7 9 1
8 7 10 1
9 7 10 1
[ dihedrals ]
3 1 2 11 3
4 1 2 11 3
5 1 2 11 3
1 2 11 14 3
1 2 11 12 3
1 2 11 13 3
2 11 14 6 3
2 11 14 15 3
2 11 14 16 3
12 11 14 6 3
12 11 14 15 3

```
 12   11   14   16     3
 13   11   14    6     3
 13   11   14   15     3
 13   11   14   16     3
 11   14    6    7     3
 15   14    6    7     3
 16   14    6    7     3
 14    6    7    8     3
 14    6    7    9     3
 14    6    7   10     3
[ pairs ]
  1   14     1
  1   12     1
  1   13     1
  2    6     1
  2   15     1
  2   16     1
 11    3     1
 11    4     1
 11    5     1
 11    7     1
 14    8     1
 14    9     1
 14   10     1
  6   12     1
  6   13     1
  7   15     1
  7   16     1
 12   15     1
 12   16     1
 13   15     1
 13   16     1
```

## E. GROMACS Forcefield parameters for all considered salt-anions:

1. $NO_3^-$

```
[ atomtypes ]
no3_001   N   7   14.00670   0.794    A   3.15000e-01  7.11280e-01
no3_002   O   8   15.99940   -0.598   A   2.86000e-01  8.78640e-01
[ atoms ]
1   no3_001   1   NOX   N   1   0.794    14.007
2   no3_002   1   NOX   O   1   -0.598   15.999
3   no3_002   1   NOX   O   1   -0.598   15.999
4   no3_002   1   NOX   O   1   -0.598   15.999
[ bonds ]
1   2   1   0.1256   530698.560
1   3   1   0.1256   530698.560
1   4   1   0.1256   530698.560
[ angles ]
2   1   3   1   120.0  1011.022
2   1   4   1   120.0  1011.022
3   1   4   1   120.0  1011.022
[ dihedrals ]
2   1   3   4   5   0.000   8.368   0.000   0.000
3   1   2   4   5   0.000   8.368   0.000   0.000
4   1   2   3   5   0.000   8.368   0.000   0.000
```

2. $BF_4^-$

```
[ atomtypes ]
bf4_001   B   5   10.811   0.8276    A  3.5814e-01   3.9748e-01
bf4_002   F   9   18.998   -0.4569   A  3.1181e-01   2.5104e-01
[ atoms ]
1   bf4_001   1   BFX   B   1   0.8276    10.811
2   bf4_002   1   BFX   F   1   -0.4569   18.998
3   bf4_002   1   BFX   F   1   -0.4569   18.998
4   bf4_002   1   BFX   F   1   -0.4569   18.998
5   bf4_002   1   BFX   F   1   -0.4569   18.998
[ bonds ]
1   2   1   0.1394   323500.000
1   3   1   0.1394   323500.000
1   4   1   0.1394   323500.000
1   5   1   0.1394   323500.000
[ angles ]
3   1   2   1   109.47  669.5
4   1   2   1   109.47  669.5
4   1   3   1   109.47  669.5
5   1   2   1   109.47  669.5
5   1   3   1   109.47  669.5
5   1   4   1   109.47  669.5
```

3. OTF ($CF_3SO_3^-$)

```
[ atomtypes ]
```

```
tfo_001   SO  16    32.064     1.020      A   0.355     1.04600
tfo_002   OS   8    15.9994   -0.630      A   0.296     0.87864
tfo_003   FC   9    18.9984   -0.160      A   0.295     0.22175
tfo_004   CF   6    12.011     0.350      A   0.350     0.27614
[ bondtypes ]
CF   FC   1   0.1323   369700
CF   SO   1   0.1818   197000
SO   OS   1   0.1442   533100
[ angletypes ]
OS  SO   OS   1    115.3   969
FC  CF   FC   1    107.1   781
FC  CF   SO   1    111.8   694
CF  SO   OS   1    102.6   870
[ dihedraltypes ]
OS  SO  CF  FC  5    0.0000    0.0000     1.4510     0.0000
[ atoms ]
1      tfo_004    1    TFO    CF    1     0.350     12.011
2      tfo_003    1    TFO    FC    2    -0.160     18.998
3      tfo_003    1    TFO    FC    2    -0.160     18.998
4      tfo_003    1    TFO    FC    2    -0.160     18.998
5      tfo_001    1    TFO    SO    3     1.020     32.066
6      tfo_002    1    TFO    OS    4    -0.630     15.999
7      tfo_002    1    TFO    OS    4    -0.630     15.999
8      tfo_002    1    TFO    OS    4    -0.630     15.999
[ pairs ]
3  8  1
3  6  1
3  7  1
4  7  1
4  6  1
2  7  1
2  6  1
2  8  1
[ bonds ]
1    2    1
1    3    1
1    4    1
1    5    1
5    6    1
5    7    1
5    8    1
[ angles ]
2  1  3  1
2  1  4  1
3  1  4  1
2  1  5  1
3  1  5  1
4  1  5  1
6  5  7  1
6  5  8  1
```

7 5 8 1
1 5 6 1
1 5 7 1
1 5 8 1
[ dihedrals ]
6 5 1 2 5
6 5 1 3 5
6 5 1 4 5
7 5 1 2 5
7 5 1 3 5
7 5 1 4 5
8 5 1 2 5
8 5 1 3 5
8 5 1 4 5

4. TFSI ($(CF_3SO_2)_2N^-$)

[ atomtypes ]
tfs_001 SO 16 32.064 1.020 A 0.355 1.04600
tfs_002 OS 8 15.9994 -0.530 A 0.296 0.87864
tfs_003 FC 9 18.9984 -0.160 A 0.295 0.22175
tfs_004 CF 6 12.011 0.350 A 0.350 0.27614
tfs_005 NI 7 14.0027 -0.660 A 0.325 0.71128
[ bondtypes ]
CF FC 1 0.1323 369700
CF SO 1 0.1818 197000
SO OS 1 0.1442 533100
NI SO 1 0.1570 311300
[ angletypes ]
OS SO OS 1 118.5 969
OS SO NI 1 113.6 789
CF SO NI 1 100.2 816
SO NI SO 1 125.6 671
FC CF FC 1 107.1 781
FC CF SO 1 111.8 694
CF SO OS 1 102.6 870
[ dihedraltypes ]
OS SO CF FC 5 0.0000 0.0000 1.4510 0.0000
NI SO CF FC 5 0.0000 0.0000 1.3220 0.0000
OS SO NI SO 5 0.0000 0.0000 -0.0150 0.0000
SO NI SO CF 5 32.7730 -10.4200 -3.1950 0.0000
[ atoms ]
1 tfs_005 1 TFS N 1 -0.660 14.0067
2 tfs_001 1 TFS S 2 1.020 32.06
3 tfs_001 1 TFS S 3 1.020 32.06
4 tfs_002 1 TFS O 4 -0.530 15.999
5 tfs_002 1 TFS O 5 -0.530 15.999
6 tfs_002 1 TFS O 6 -0.530 15.999
7 tfs_002 1 TFS O 7 -0.530 15.999
8 tfs_004 1 TFS C 8 0.350 12.011

9 tfs_004 1 TFS C 9 0.350 12.011
10 tfs_003 1 TFS F 10 -0.160 18.9984
11 tfs_003 1 TFS F 11 -0.160 18.9984
12 tfs_003 1 TFS F 12 -0.160 18.9984
13 tfs_003 1 TFS F 13 -0.160 18.9984
14 tfs_003 1 TFS F 14 -0.160 18.9984
15 tfs_003 1 TFS F 15 -0.160 18.9984
[ bonds ]
1 2 1
1 3 1
2 6 1
2 7 1
2 9 1
3 8 1
3 4 1
3 5 1
8 10 1
8 11 1
8 12 1
9 13 1
9 14 1
9 15 1
[ angles ]
13 9 14 1
13 9 15 1
14 9 15 1
13 9 2 1
14 9 2 1
15 9 2 1
9 2 6 1
9 2 7 1
9 2 1 1
2 1 3 1
6 2 1 1
7 2 1 1
1 3 4 1
1 3 5 1
1 3 8 1
4 3 8 1
5 3 8 1
3 8 10 1
3 8 11 1
3 8 12 1
10 8 11 1
10 8 12 1
11 8 12 1
6 2 7 1
4 3 5 1
[ dihedrals ]
3 1 2 6 5 ; S-N-S-O

| | | | | |
|---|---|---|---|---|
| 3 | 1 | 2 | 7 | 5 |
| 2 | 1 | 3 | 4 | 5 |
| 2 | 1 | 3 | 5 | 5 |
| 1 | 3 | 8 | 10 | 5 |
| 1 | 3 | 8 | 11 | 5 |
| 1 | 3 | 8 | 12 | 5 |
| 1 | 2 | 9 | 13 | 5 |
| 1 | 2 | 9 | 14 | 5 |
| 1 | 2 | 9 | 15 | 5 |
| 5 | 3 | 8 | 10 | 5 |
| 5 | 3 | 8 | 11 | 5 |
| 5 | 3 | 8 | 12 | 5 |
| 4 | 3 | 8 | 10 | 5 |
| 4 | 3 | 8 | 11 | 5 |
| 4 | 3 | 8 | 12 | 5 |
| 6 | 2 | 9 | 13 | 5 |
| 6 | 2 | 9 | 14 | 5 |
| 6 | 2 | 9 | 15 | 5 |
| 7 | 2 | 9 | 13 | 5 |
| 7 | 2 | 9 | 14 | 5 |
| 7 | 2 | 9 | 15 | 5 |
| 3 | 1 | 2 | 9 | 5 |
| 2 | 1 | 3 | 8 | 5 |

[ pairs ]

| | | |
|---|---|---|
| 2 | 4 | 1 |
| 2 | 5 | 1 |
| 3 | 6 | 1 |
| 3 | 7 | 1 |
| 10 | 4 | 1 |
| 11 | 4 | 1 |
| 12 | 4 | 1 |
| 10 | 5 | 1 |
| 11 | 5 | 1 |
| 12 | 5 | 1 |
| 1 | 10 | 1 |
| 1 | 11 | 1 |
| 1 | 12 | 1 |
| 8 | 2 | 1 |
| 9 | 3 | 1 |
| 13 | 6 | 1 |
| 14 | 6 | 1 |
| 15 | 6 | 1 |
| 13 | 7 | 1 |
| 14 | 7 | 1 |
| 15 | 7 | 1 |
| 13 | 1 | 1 |
| 14 | 1 | 1 |
| 15 | 1 | 1 |
